# Supplementary material for: STEEX: Steering Counterfactual Explanations with Semantics
Source: arXiv:2111.09094 source file (2022-07-18)
Supplement: Supplementary file 1 [file suppl_celebamhq_b.pdf]

Query image

Reconstruct.

STEEEX (ours)

Smile

Young

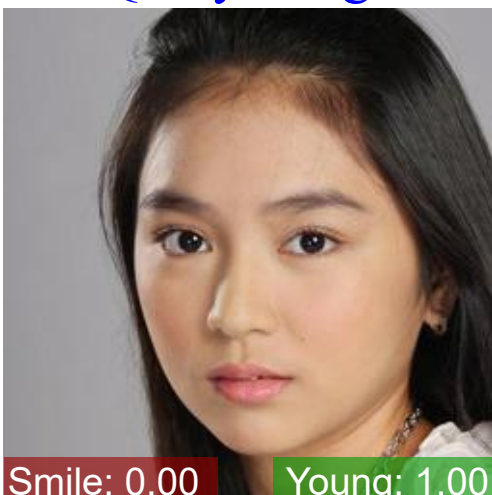

Smile: 0.00 Young: 1.00

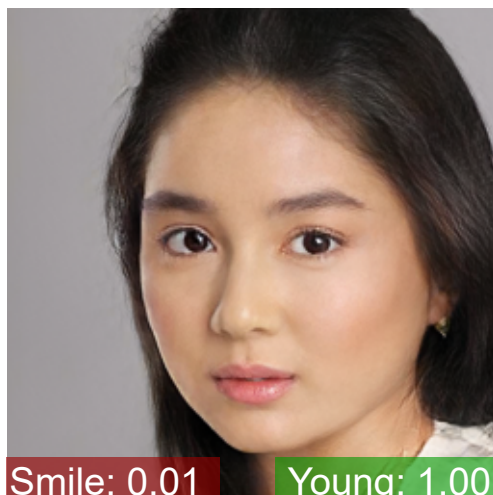

Smile: 0.01 Young: 1.00

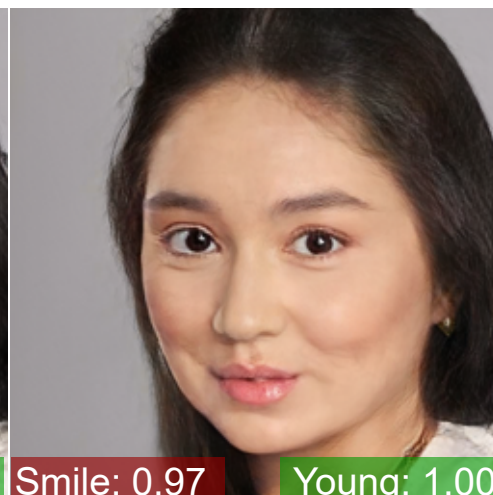

Smile: 0.97 Young: 1.00

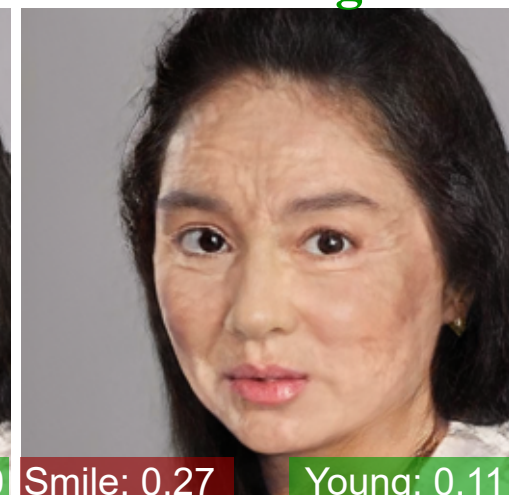

Smile: 0.27 Young: 0.11

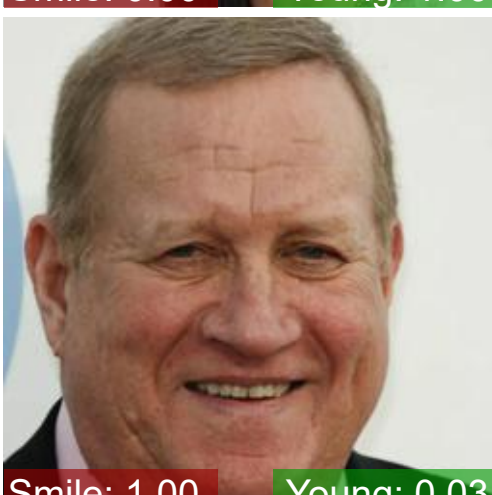

Smile: 1.00 Young: 0.03

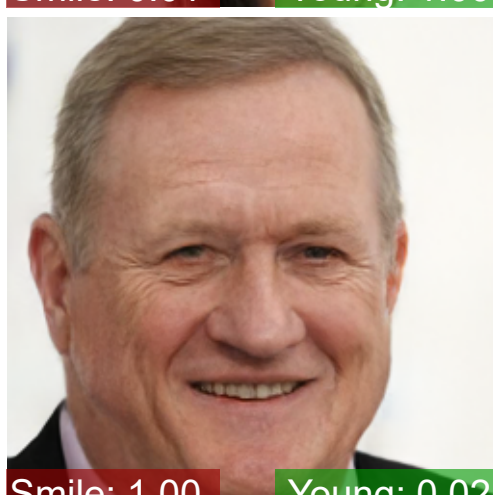

Smile: 1.00 Young: 0.02

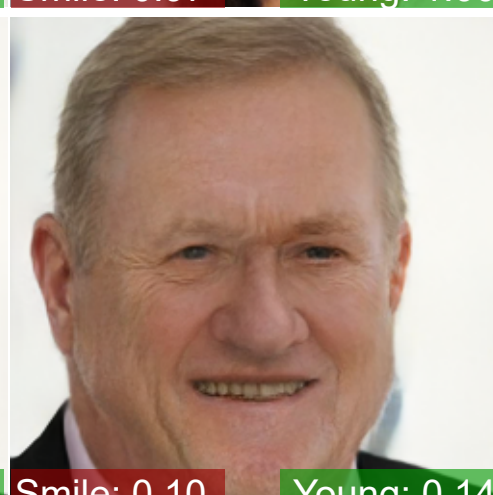

Smile: 0.10 Young: 0.14

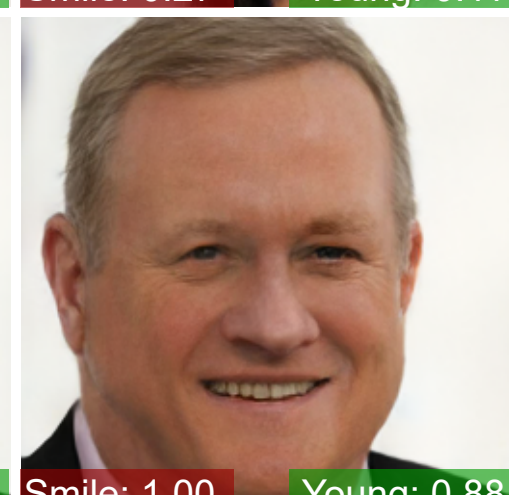

Smile: 1.00 Young: 0.88

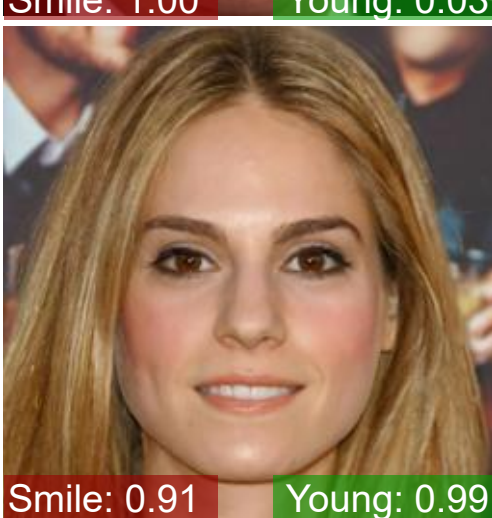

Smile: 0.91 Young: 0.99

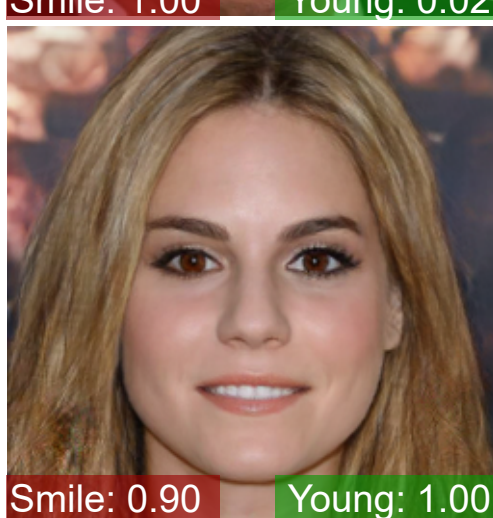

Smile: 0.90 Young: 1.00

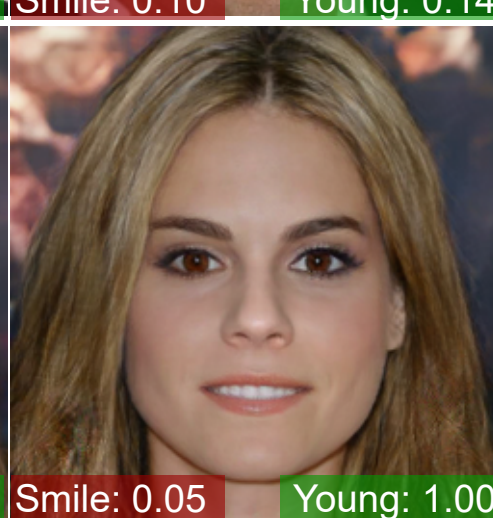

Smile: 0.05 Young: 1.00

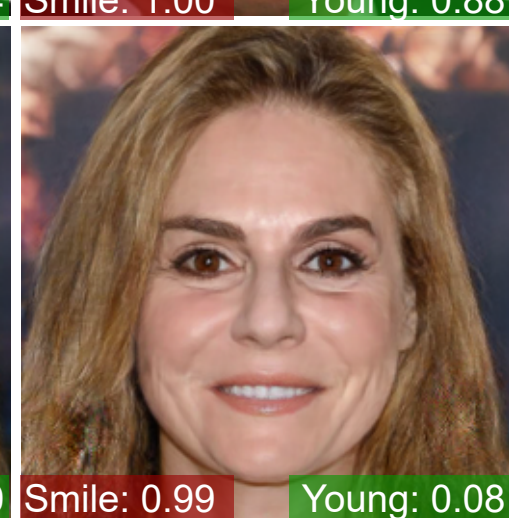

Smile: 0.99 Young: 0.08

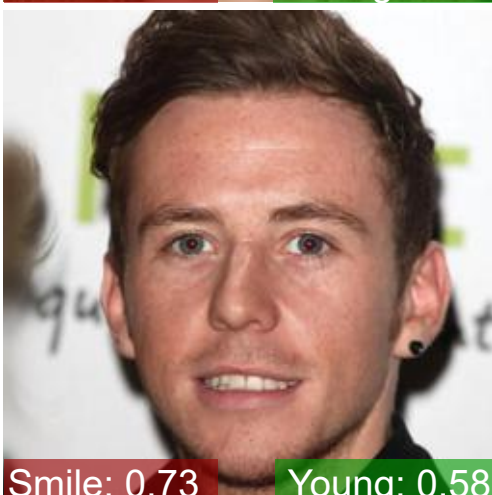

Smile: 0.73 Young: 0.58

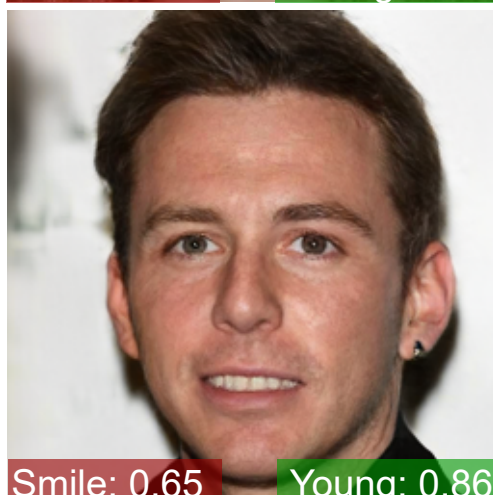

Smile: 0.65 Young: 0.86

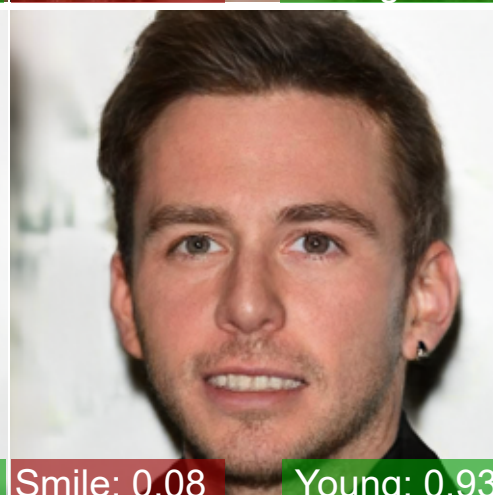

Smile: 0.08 Young: 0.93

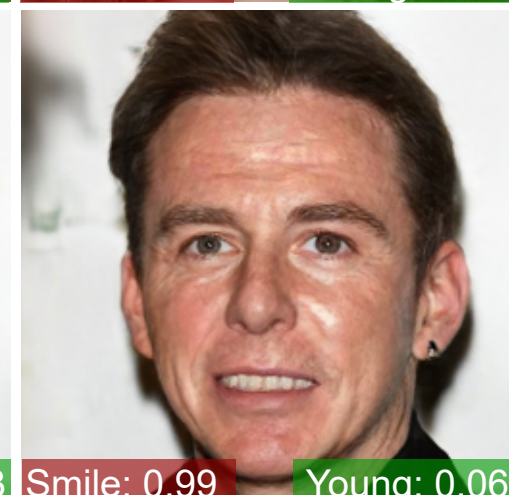

Smile: 0.99 Young: 0.06

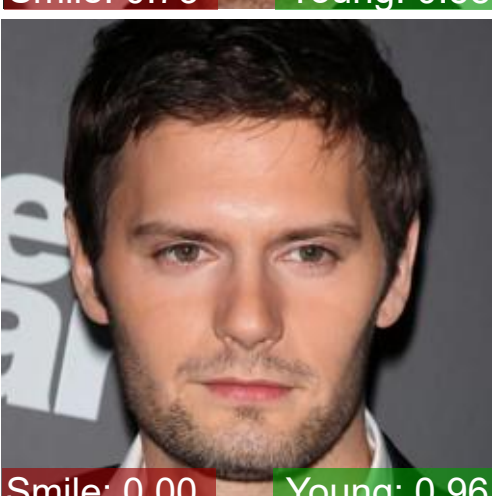

Smile: 0.00 Young: 0.96

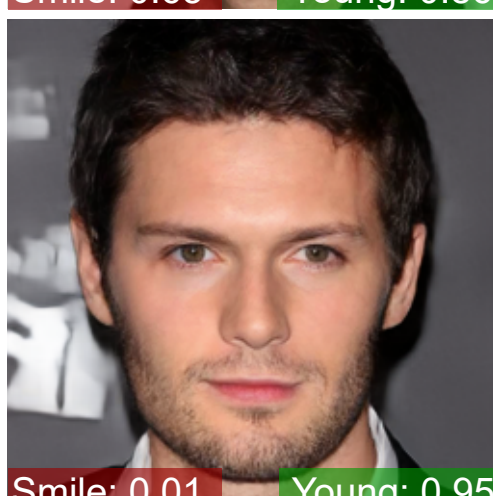

Smile: 0.01 Young: 0.95

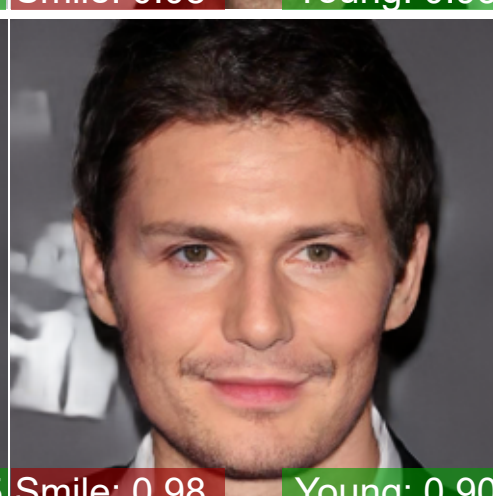

Smile: 0.98 Young: 0.90

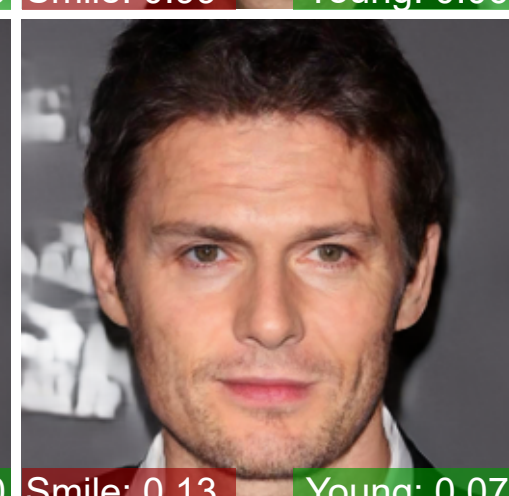

Smile: 0.13 Young: 0.07
